# Supplementary material for: AllClear: A Comprehensive Dataset and Benchmark for Cloud Removal in Satellite Imagery
Source: arXiv:2410.23891 source file (2024-10-31)
Supplement: Supplementary file 1 [file 6_appendix.tex]

\newpage
\appendix
\input{s1_overview}

\input{s3_dataset}
\input{s4_experiments}
\input{s2_datasheet}
